# Supplementary material for: The GALAH Survey: Chemical tagging and chrono-chemodynamics of accreted halo stars with GALAH+ DR3 and $Gaia$ eDR3
Source: arXiv:2109.04059 source file (2022-01-06)
Supplement: Supplementary file 1 [file above_84thchem_Si_fe.tex]

29\%%
