# Supplementary material for: The GALAH Survey: Chemical tagging and chrono-chemodynamics of accreted halo stars with GALAH+ DR3 and $Gaia$ eDR3
Source: arXiv:2109.04059 source file (2022-01-06)
Supplement: Supplementary file 2 [file trace_stats_Mg_Si.tex]

$\mathrm{[Mg/Si]} = 0.02_{-0.10}^{+0.13}$,
